# Supplementary material for: Leveraging Smooth Attention Prior for Multi-Agent Trajectory Prediction
Source: arXiv:2203.04421 source file (2022-03-19)
Supplement: Supplementary file 1 [file appendix.tex]

%%%%%%%%%%%%%%%%%%%%%%%%%%%%%%%%%%%%%%%%%%%%%%%%%%%%%%%%%%%%%%%%%%%%%%%%%%%%%%%%
%2345678901234567890123456789012345678901234567890123456789012345678901234567890
%        1         2         3         4         5         6         7         8

%\documentclass[letterpaper, 10 pt, conference]{ieeeconf}  % Comment this line out if you need a4paper
\documentclass[letterpaper, 10 pt, journal, twoside]{IEEEtran}

\IEEEoverridecommandlockouts                              % This command is only needed if 
                                                          % you want to use the \thanks command

%\overrideIEEEmargins                                      % Needed to meet printer requirements.

%In case you encounter the following error:
%Error 1010 The PDF file may be corrupt (unable to open PDF file) OR
%Error 1000 An error occurred while parsing a contents stream. Unable to analyze the PDF file.
%This is a known problem with pdfLaTeX conversion filter. The file cannot be opened with acrobat reader
%Please use one of the alternatives below to circumvent this error by uncommenting one or the other
%\pdfobjcompresslevel=0
%\pdfminorversion=4

% See the \addtolength command later in the file to balance the column lengths
% on the last page of the document

% Paper headers
\markboth{IEEE Robotics and Automation Letters. Preprint Version. Accepted February, 2021}
{Cao \MakeLowercase{\textit{et al.}}: Leveraging Temporal Structures in Attention\\for Multi-Agent Trajectory Prediction} 

% The following packages can be found on http:\\www.ctan.org
\usepackage{graphics} % for pdf, bitmapped graphics files
\usepackage{epsfig} % for postscript graphics files
\usepackage{times} % assumes new font selection scheme installed
\usepackage{amsmath} % assumes amsmath package installed
\usepackage{amssymb}  % assumes amsmath package installed

\usepackage{multicol}
\usepackage{graphicx}
\usepackage{bm,amsfonts}
\usepackage{subfigure}
\usepackage{xcolor}
\usepackage{hyperref}
\hypersetup{
    colorlinks=true,
    linkcolor=orange,
    filecolor=magenta,      
    urlcolor=orange,
    citecolor=orange,
}
\usepackage[style=numeric,sorting=none]{biblatex}
\usepackage{balance}

\addbibresource{references.bib}

\title{\LARGE \bf Leveraging Temporal Structures in Attention\\for Multi-Agent Trajectory Prediction}

\author{Zhangjie Cao$^1$, Erdem B\i y\i k$^2$, Guy Rosman$^3$, Dorsa Sadigh$^{1,2}$%
    \thanks{Emails: {\tt\footnotesize caozj@cs.stanford.edu, ebiyik@stanford.edu, guy.rosman@tri.global, dorsa@cs.stanford.edu}}%
    \thanks{$^1$Computer Science, Stanford University, CA, USA}%
    \thanks{$^2$Electrical Engineering, Stanford University, CA, USA}%
    \thanks{$^3$Toyota Research Institute, MA, USA}%
    }

\begin{document}

\maketitle

\renewcommand*{\bibfont}{\small}
\balance\printbibliography

\end{document}
